# Supplementary material for: Emergence of Symbols in Neural Networks for Semantic Understanding and Communication
Source: arXiv:2304.06377 ancillary file (2023-06-25)
Supplement: Supplementary file 1 [file Supplementary_Materials.pdf]

Supplementary Materials for

# Emergence of Symbols in Neural Networks for Semantic Understanding and Communication

Yang Chen *et al.*

*Corresponding author. Email: yang.chen@ia.ac.cn (Y.C.), shan.yu@nlpr.ia.ac.cn (S.Y.)

**This PDF file includes:**

Figs. S1 to S3
Tables S1

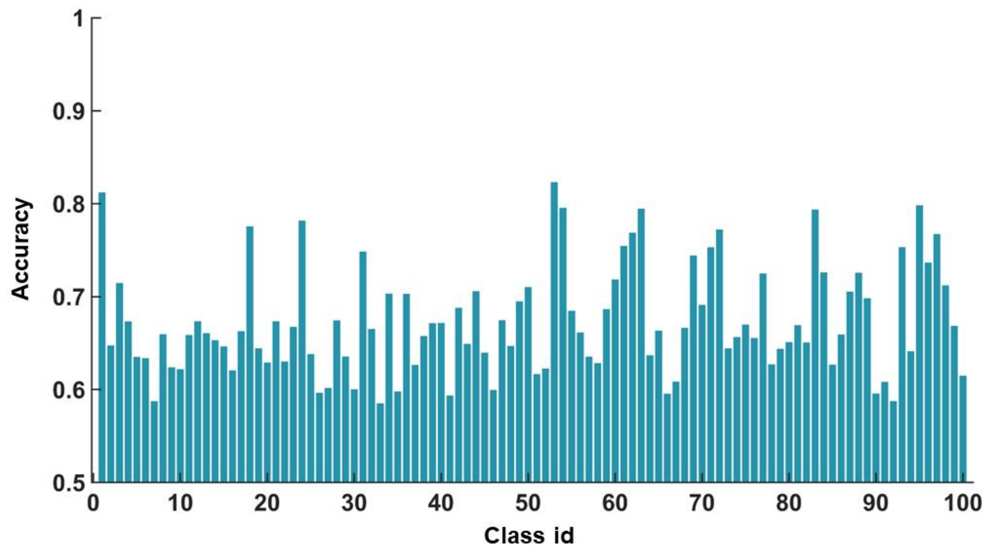


**Figure S1. The performance of SEA-net on the symbolically inferred classes**.

SEA-net can achieve identification accuracy much higher than the chance level (0.5) by purely modifying symbolic inputs it received.

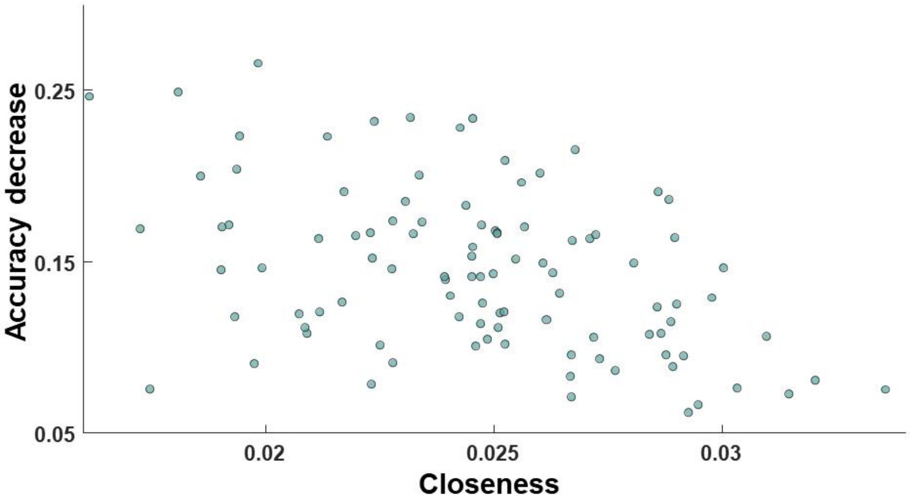


**Figure S2. Influence of the semantic structure on the identification accuracy for symbolically inferred classes.** The scatter plot between closeness and identification accuracy decrease for individual classes (green dots) is shown. The accuracy decrease was measured by $(ACC\text{-}ACC_{si})/ ACC$, where ACC is the identification accuracy achieved with standard training (cf. Fig. 1D) and $ACC_{si}$ is the accuracy achieved through symbolically inferring (cf. Fig. S1). The closeness of each class was measured by how its corresponding symbol (generated by SEA-net) related to other symbols. Precisely, it was calculated as the reciprocal of the average shortest path length of individual symbols in the network constructed based on the cosine distance matrix (Fig. 2A), in which nodes represent symbols and edge strength represents the cosine distance between symbols.

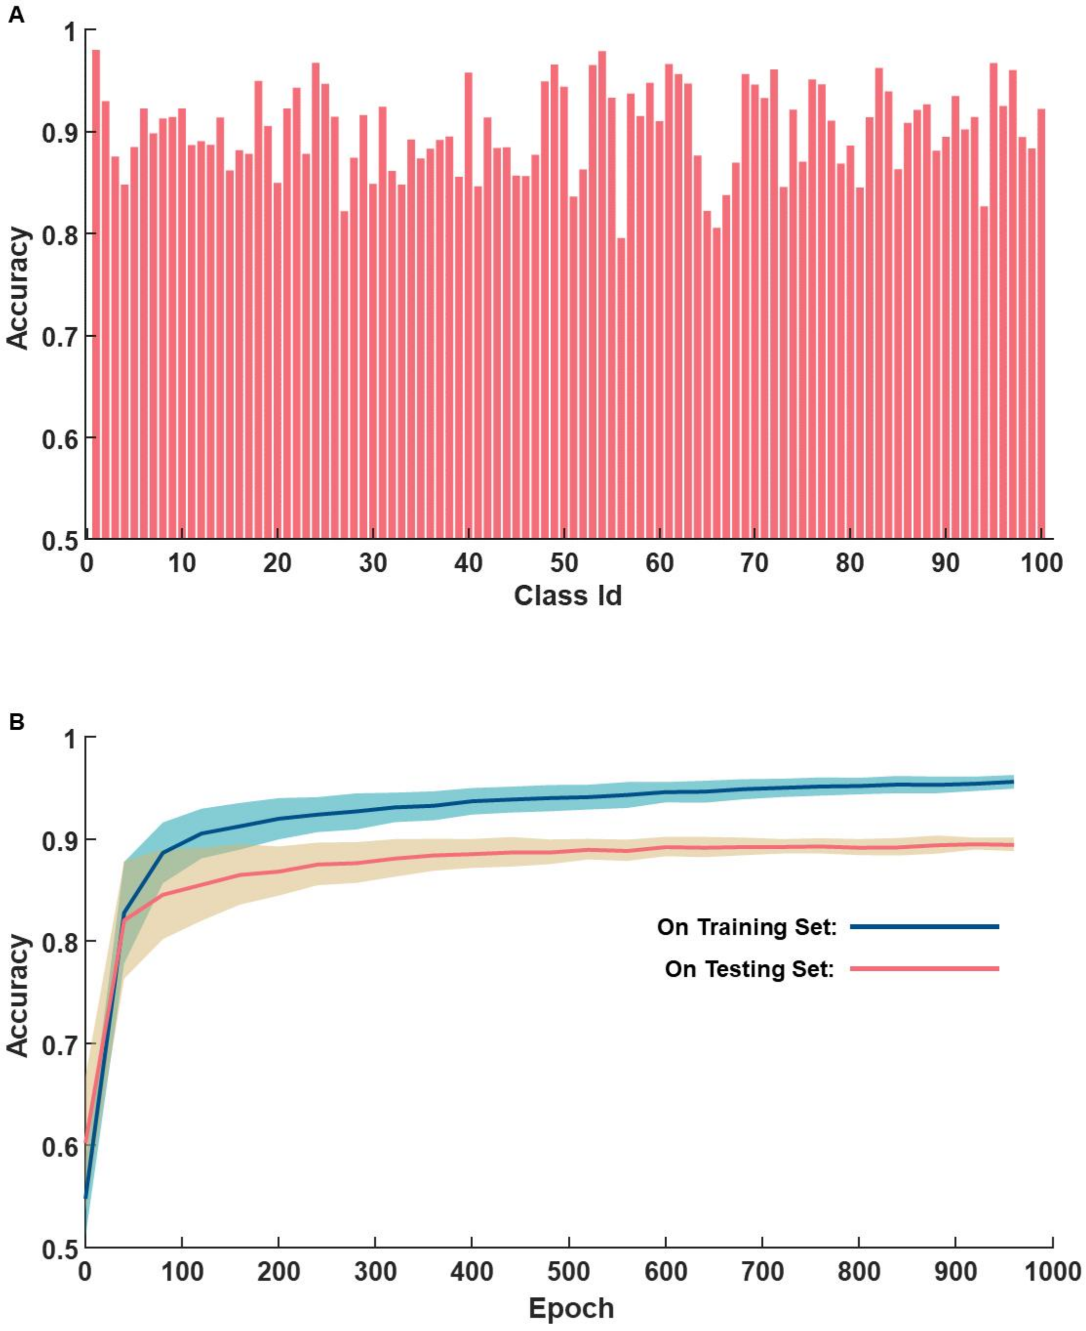


**Figure S3. The identification accuracy of SEA-net with a trainable feature extractor in the learning process**. (A) The testing accuracy of each class in CIFAR 100 was achieved by the SEA-net with a trainable feature extractor. (B) The performance of SEA-net during the training process. The green line represents the

accuracy during the training, while the orange line represents the accuracy during the testing.

**Table S1.** Category IDs in CIFAR 100 and corresponding names.

| Category ID | Category Name | Category ID | Category Name |
|---|---|---|---|
| 1 | apple | 51 | mouse |
| 2 | aquarium fish | 52 | mushroom |
| 3 | baby | 53 | oak tree |
| 4 | bear | 54 | orange |
| 5 | beaver | 55 | orchid |
| 6 | bed | 56 | otter |
| 7 | bee | 57 | palm tree |
| 8 | beetle | 58 | pear |
| 9 | bicycle | 59 | pickup truck |
| 10 | bottle | 60 | pine tree |
| 11 | bowl | 61 | plain |
| 12 | boy | 62 | plate |
| 13 | bridge | 63 | poppy |
| 14 | bus | 64 | porcupine |
| 15 | butterfly | 65 | possum |
| 16 | camel | 66 | rabbit |
| 17 | can | 67 | raccoon |
| 18 | castle | 68 | ray |
| 19 | caterpillar | 69 | road |
| 20 | cattle | 70 | rocket |
| 21 | chair | 71 | rose |
| 22 | chimpanzee | 72 | sea |
| 23 | clock | 73 | seal |
| 24 | cloud | 74 | shark |
| 25 | cockroach | 75 | shrew |
| 26 | couch | 76 | skunk |
| 27 | cra | 77 | skyscraper |
| 28 | crocodile | 78 | snail |
| 29 | cup | 79 | snake |
| 30 | dinosaur | 80 | spider |
| 31 | dolphin | 81 | squirrel |
| 32 | elephant | 82 | streetcar |
| 33 | flatfish | 83 | sunflower |
| 34 | forest | 84 | sweet pepper |

| | | | |
|---|---|---|---|
| 35 | fox | 85 | table |
| 36 | girl | 86 | tank |
| 37 | hamster | 87 | telephone |
| 38 | house | 88 | television |
| 39 | kangaroo | 89 | tiger |
| 40 | keyboard | 90 | tractor |
| 41 | lamp | 91 | train |
| 42 | lawn mower | 92 | trout |
| 43 | leopard | 93 | tulip |
| 44 | lion | 94 | turtle |
| 45 | lizard | 95 | wardrobe |
| 46 | lobster | 96 | whale |
| 47 | man | 97 | willow tree |
| 48 | maple tree | 98 | wolf |
| 49 | motorcycle | 99 | woman |
| 50 | mountain | 100 | worm |
